# Supplementary material for: Deep-ER: Deep Learning ECCENTRIC Reconstruction for fast high-resolution neurometabolic imaging
Source: arXiv:2409.18303 source file (2025-12-15)
Supplement: Supplementary file 1 [file neuroimage-supplementary.tex]

\documentclass[../neuroimage-main.tex]{subfiles}

\myexternaldocument{sections/neuroimage-article}

\begin{document}

%\title{Supplementary Material to \textit{"\deep{}: Deep Learning ECCENTRIC Reconstruction for fast high-resolution neurometabolic imaging"}}

\centering{\Huge{\textbf{Supplementary Material}}}
\renewcommand{\figurename}{\textbf{Supplementary Figure}}
\setcounter{figure}{0}

\justifying
\section{Supplementary Methods}

\subsection{MRSI pre-processing:} \label{subsec:methods:MRSIpreproc}
MRSI 4D (k,t) data of each coil channel were pre-processed by applying Hamming filter and density compensation based on Voronoi diagrams \cite{malik2005gridding}. Voronoi diagrams were computed based on the ECCENTRIC sampling scheme and each k-space points was normalized by the area of its assigned Voronoi vertex. Inverse non-uniform Fourier transform (iNUFT) \cite{bagchi1996nonuniform} was performed with the density compensation for each in-plane partition ($k_x$,$k_y$) and conventional inverse fast Fourier transformation was applied along the uniformly sampled $k_z$ axis. 

Coil combination was performed by multiplication of the adjoint coil sensitivity profile with each channel and their summation, resulting in the initial 4D image-time MRSI data. Coil sensitivity profiles were computed from water un-suppressed MRSI data using ESPIRiT \cite{uecker2014espirit}. 

To compensate for $B_0$ field inhomogeneities, a frequency shift map was estimated from water un-suppressed measurement and applied on the coil combined MRSI image \cite{klauser2021achieving}.

Water residual was removed using Hankel singular value decomposition \cite{cabanes2001optimization} and filtering out frequencies from a predefined range around $4.7$ppm.

\subsection{Deep Learning Lipid Removal:}
Before  DL reconstruction of the MRSI dataset, the nuisance lipid signal was removed by a new approach using deep learning to identify the lipid signal. The WALINET (WAter and LIpid neural NETwork) method provides an improvement over the conventional L2-lipid regularization suppression method \cite{bilgic2014fast}. 

The network architecture was based on Y-Net \cite{mohammed2018net} with 2 encoders and 1 decoder. The encoders and decoders consist of 4 convolutional blocks followed by MaxPooling or upsampling. Each convolutional block contains dropout, two convolutional layers and two ReLU activation functions. Skip connections are applied between the blocks in the encoders and decoder. Full details about WALINET are presented in \cite{weiser2024lipcon}.

\subsection{\tgv{} Reconstruction:}
A low-rank (LR) model constrained with Total-Generalized-Variation (TGV) was used for the \tgv{} reconstruction \cite{klauser2023eccentric}
 \begin{eqnarray}\label{eq:Recon}
 \arg \min_{ \mathbf{U},\mathbf{V},\mathbf{L}} & \left\| \mathcal{W}\left (\mathbf{s} - \mathcal{FCB} \left(\mathbf{U}\mathbf{V}+\mathbf{L}\right)\right ) \right\|^2_2 \nonumber\\
 &+ \lambda \sum_{c=1}^{K}\text{TGV}^2\{U_c\},
\end{eqnarray}
where $\mathbf{s}$ is the measured data, $\mathcal{F}$ the non-uniform Fourier transform (NUFT) encoding operator, $\mathcal{C}$ the coil sensitivity operator, $\mathcal{B}$ the $B_0$ frequency shift operator and $\mathbf{L}$ represents the lipid signal ($N_{\mathbf{r}}$ by $T$ array) located at the skull that is reconstructed simultaneously with spatial ($\mathbf{U}$) and temporal ($\mathbf{V}$) low-rank components of the brain metabolites signal. $\mathcal{W}$, is a weighting operator of a Hamming window shape. $\text{TGV}^2$ is the total generalized variation regularization with parameter $\lambda$ \cite{knoll2011second}.

The regularization parameter used in the reconstruction was adjusted to $ \lambda =3 \times 10^{-4}$ and $K$ was specifically set to 40, identical to the original work \cite{klauser2023eccentric}. The metabolite ECCENTRIC reconstruction described by Equation \ref{eq:Recon} is referred in this paper as \tgv{}.

The \tgv{} was employed with some modification to obtain the ground truth water image $x_{GT}$ used for training the Interlacer network (Eqs. 5-6). For this purpose, the low-rank assumption and the lipid reconstruction ($\mathbf{L}$) steps were omitted, since spectral decomposition and lipid removal is not required for the water signal. Each time-point in the water dataset was treated as an independent image and reconstructed sequentially using the \tgv{} method.

\subsection{Spectral fitting}
Spectral fitting of metabolites was performed by LCModel \cite{provencher2014lcmodel} using a basis set containing spectra simulated by NMR quantum mechanics in GAMMA (19) for twenty-two metabolites: phosphorylcholine (PCh), glycerophosphorylcholine (GPC), creatine (Cr), phosphocreatine (PCr), gamma-aminobutyric acid (GABA), glutamate (Glu), glutamine (Gln), glycine (Gly), glutathione (GSH), myo-inositol (Ins), N-acetylaspartate (NAA), N-acetyl aspartylglutamate (NAAG), scylloinositol (Sci), lactate (Lac), threonine (Thr), beta-glucose (bGlu), alanine (Ala), aspartate (Asp), ascorbate (Asc), serine (Ser), taurine (Tau), and 2-hydroxyglutarate (2HG) and a measured macromolecular background \cite{povavzan2015mapping}. The spectral fitting was done for 1ppm-4.2ppm spectral range and the results for each voxel were used to generate metabolic images. The unsupressed water signal was used as quantification reference for metabolites concentrations (institutional units, I.U.) to compare metabolite levels across subjects and scanners. To assess the quality of the MRSI data and fit, linewidth (FWHM), signal-to-noise ratio (SNR), and Cramer-Rao lower bounds (CRLB) goodness of fit maps were generated. 

\subsection{Image quality metrics}
To assess the quality of image reconstruction methods and the agreement with the ground truth the normalized root mean square error (NRMSE), correlation coefficients (CC), and the structure similarity index (SSIM) \cite{wang2004image} were calculated .  

\subsection{High resolution metabolic phantom}
A custom made high resolution metabolic phantom with geometry similar to Derenzo molecular imaging phantom \cite{derenzo1977high} contained 5 sets of tubes with diameters of 2, 4, 6, 8 and 10 mm as shown in Figure \ref{fig:phantom}. Each set contained 6 tubes of identical diameters separated by a distance equal to twice the inner diameter positioned in a triangular configuration. In every set, the six tubes were filled with metabolite solutions including 10~mM of creatine. Magnevist (Gd-DTPA) was added (1 mL/L) in each tube to shorten $T_1$ and create $T_1$-weighted contrast for structural MRI. The whole tube structure was inserted in a large cylindrical container (13.33~cm inner diameter) which was filled with 10~mM NaCl solution.  

\newpage
\section{Supplementary Results}

\begin{figure}[ht!]
    \centering
    \includegraphics[width=1\textwidth]{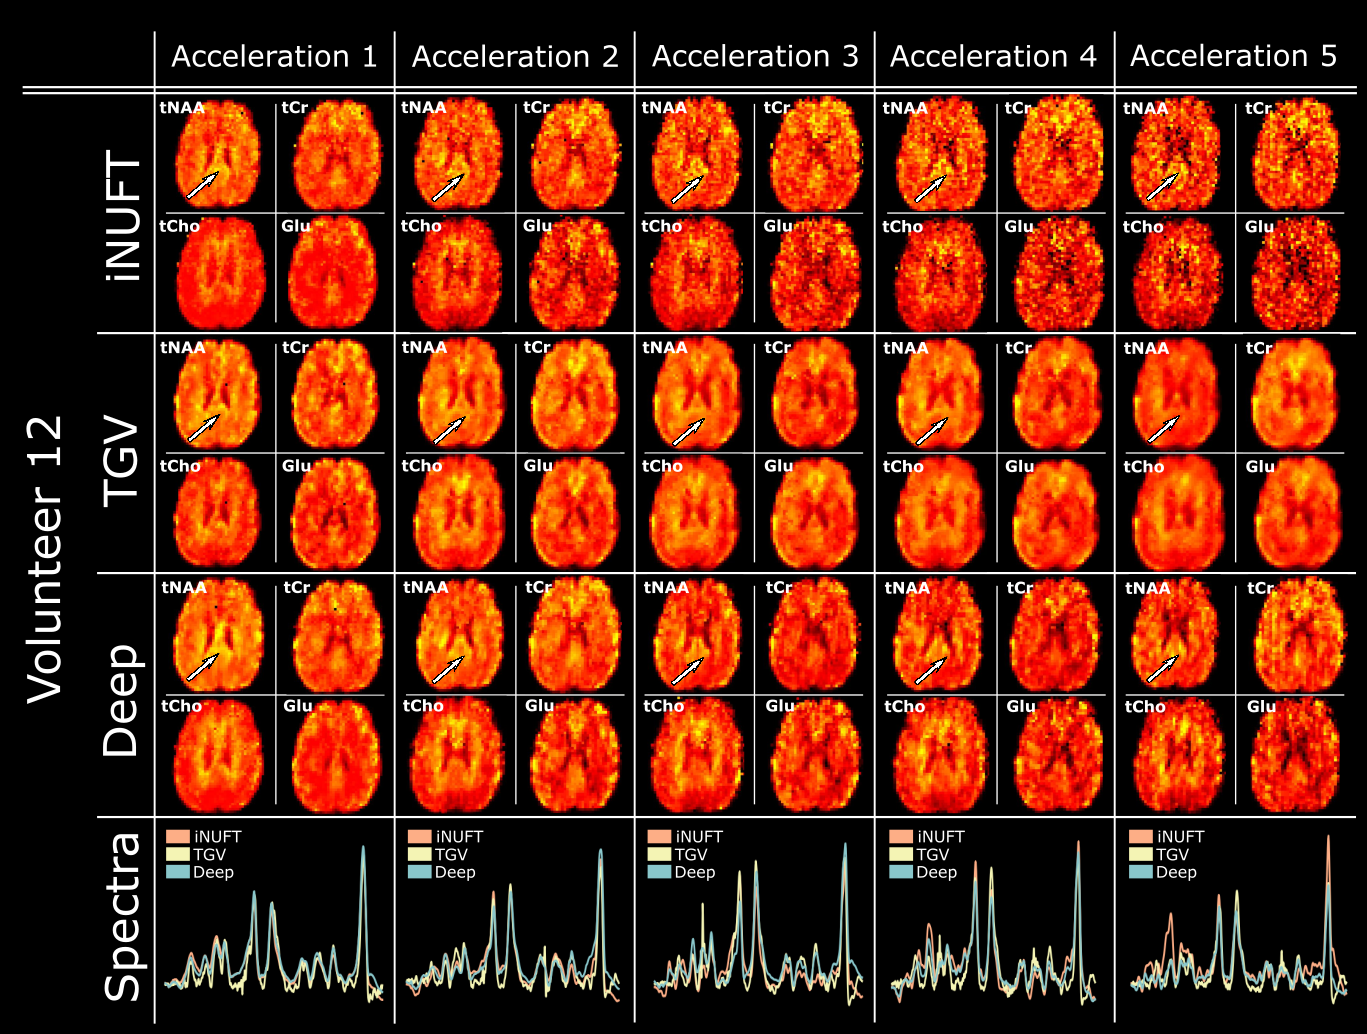}
    \caption{Comparison of different MRSI reconstruction methods across accelerations from 1 to 5. Four different metabolic maps are presented for each method and acceleration, including total NAA, total Cr, total Cho and Glu. Examples of spectra obtained by each method are shown overlaid at the bottom for each acceleration. Arrow indicate the voxel location for the spectra.}
    \label{fig:acc}
\end{figure}

\begin{figure}[ht!]
    \centering
    \includegraphics[width=1\textwidth]{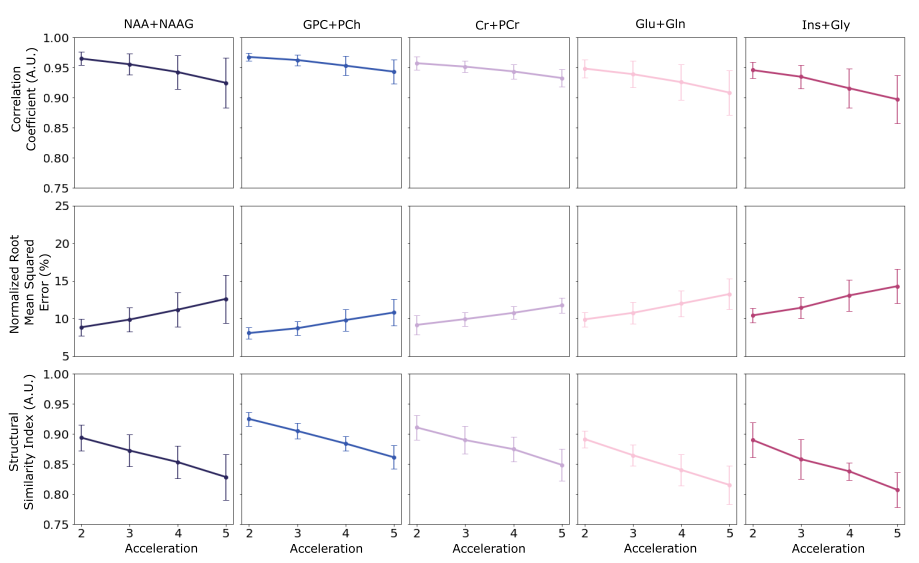}
    \caption{Quantitative comparison between \deep{} and \tgv{} showing plots of NRMSE, SSIM and Correlation Coefficient across accelerations 2 to 5 for five metabolic maps including NAA+NAAG, GPC+PCh, Cr+PCr, Glu+Gln and Ins+Gly. \green{Line plots show the mean across all subjects, and the error bar represent the standard deviation.}}
    \label{fig:acc_quant}
\end{figure}

\begin{figure}[ht!]
    \centering
    \includegraphics[width=1\textwidth]{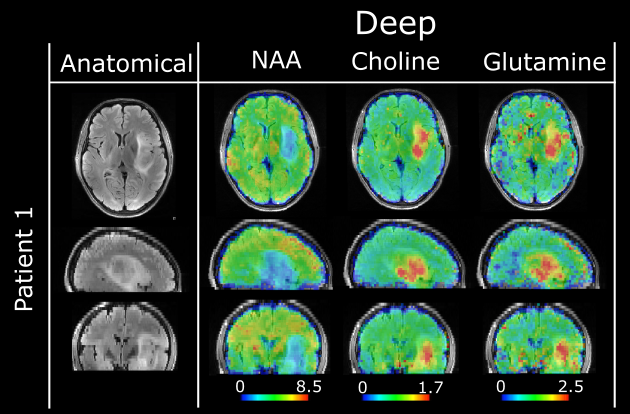}
    \caption{}
    \label{fig:qual_lowop}
\end{figure}

%\clearpage
%\printbibliography
\end{document}
